# Supplementary material for: SemIE: Semantically-aware Image Extrapolation
Source: arXiv:2108.13702 source file (2021-08-31)
Supplement: Supplementary file 1 [file semantic1.pdf]

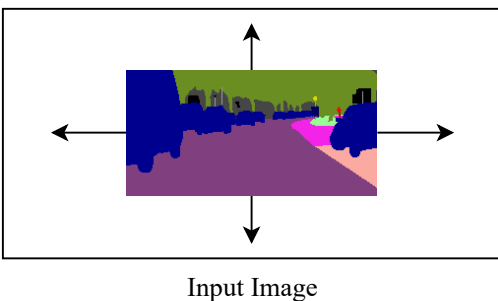

Ours w/o Boundary channel

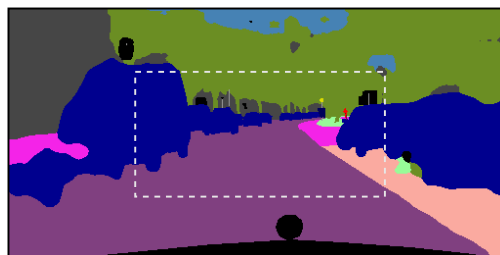

Ours

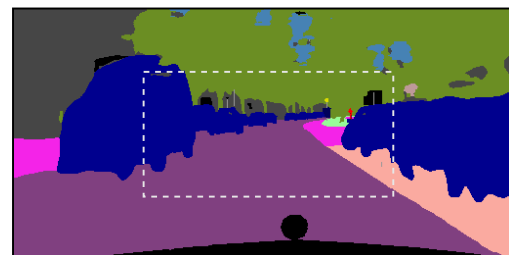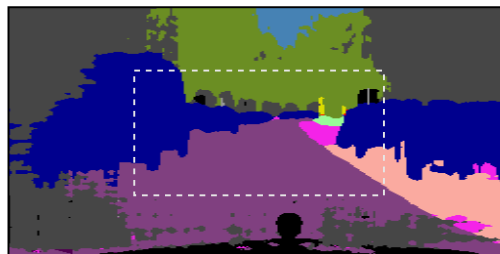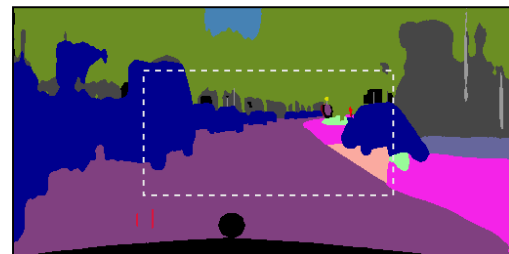

SPG-Net

SPG-Net ++

Ours w/o Boundary channel

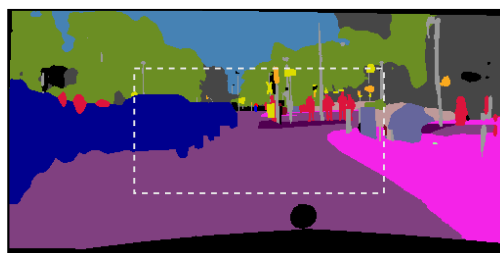

Ours

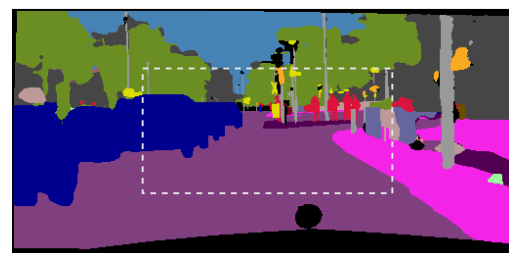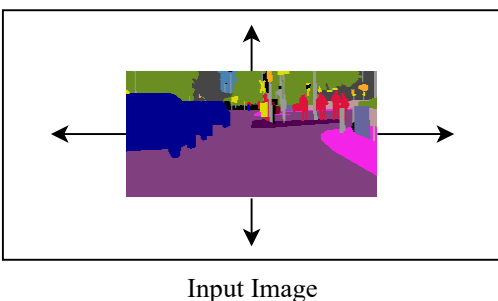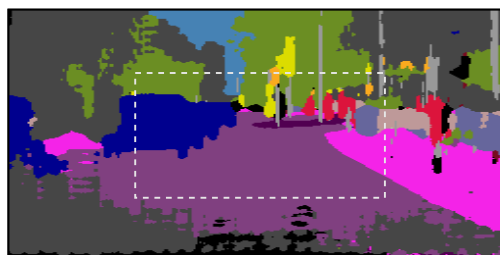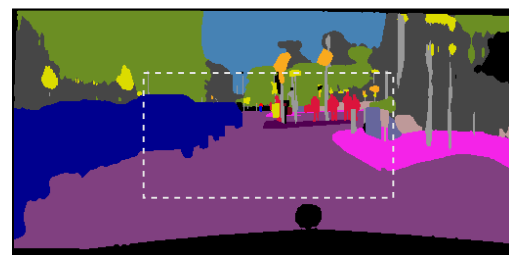

SPG-Net

SPG-Net ++

Ours w/o Boundary channel

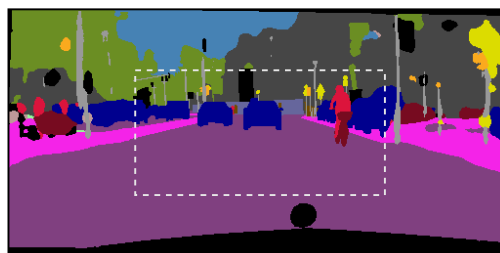

Ours

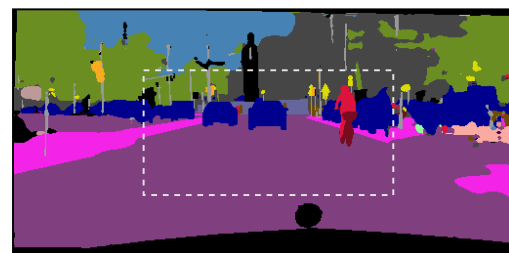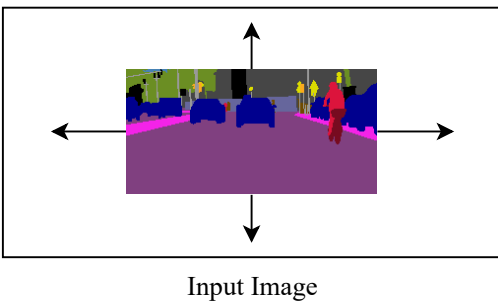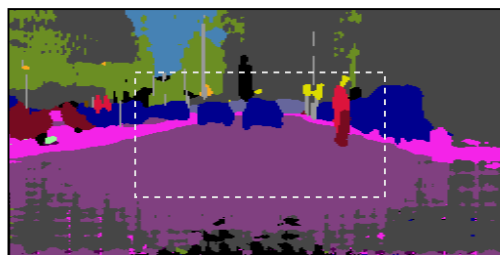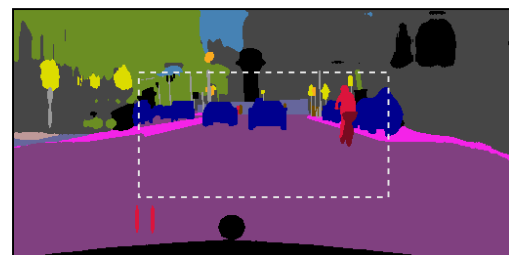

SPG-Net

SPG-Net ++
