# Supplementary material for: SemIE: Semantically-aware Image Extrapolation
Source: arXiv:2108.13702 source file (2021-08-31)
Supplement: Supplementary file 2 [file semantic2.pdf]

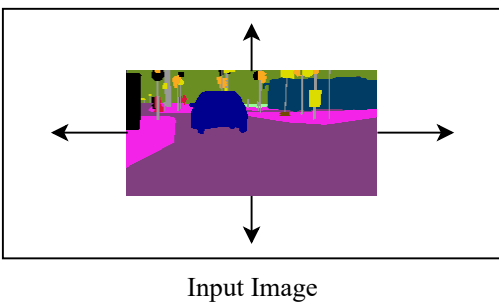

Ours w/o Boundary channel

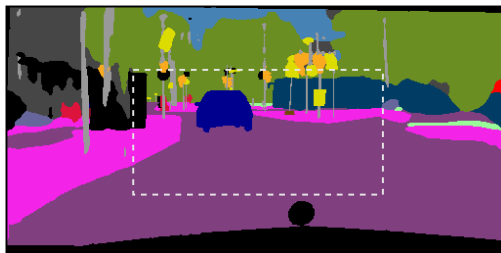

Ours

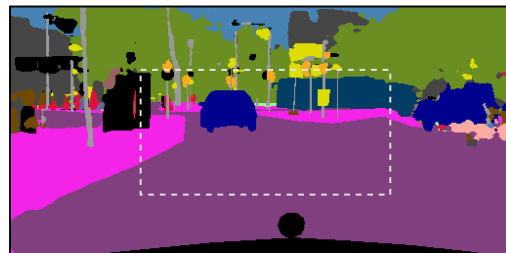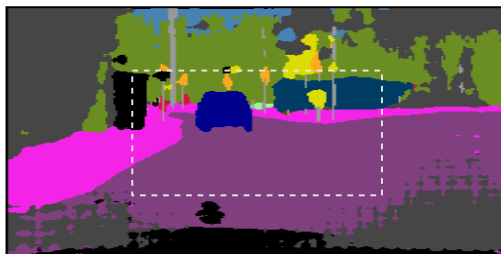

SPG-Net

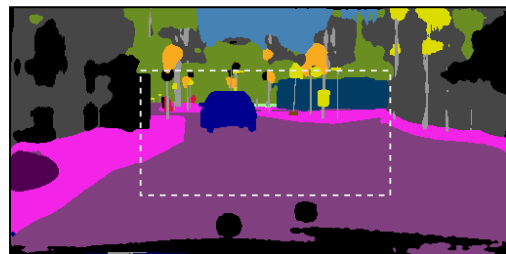

SPG-Net ++

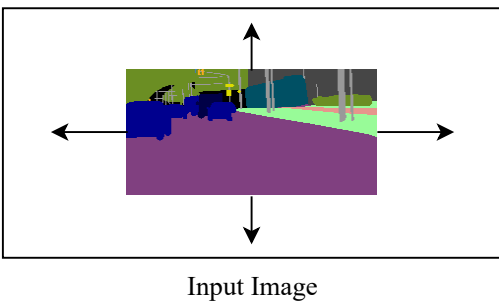

Ours w/o Boundary channel

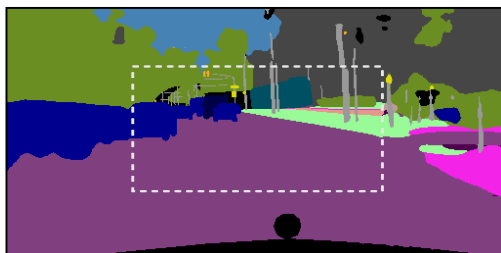

Ours

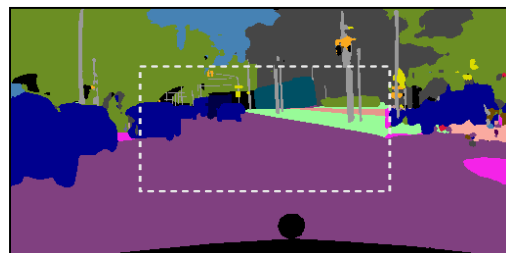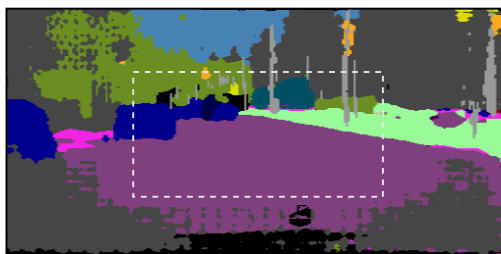

SPG-Net

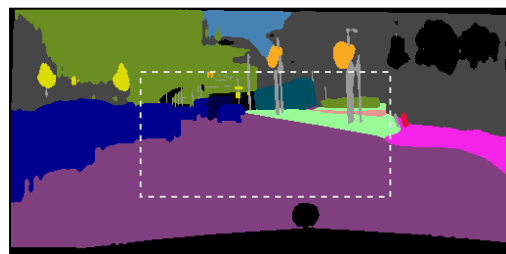

SPG-Net ++

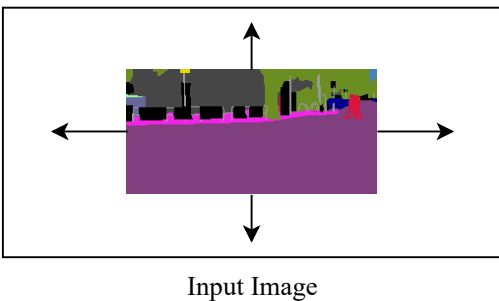

Ours w/o Boundary channel

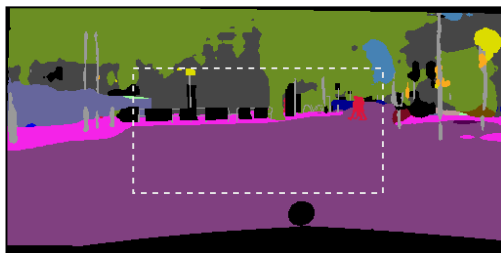

Ours

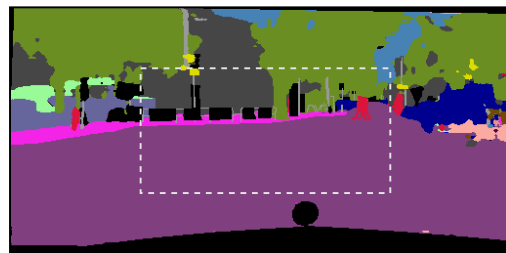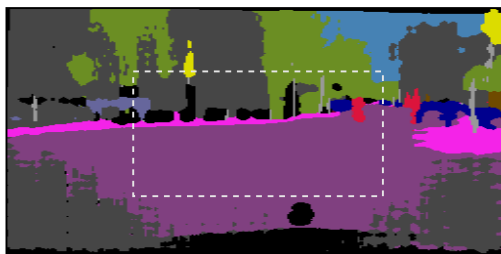

SPG-Net

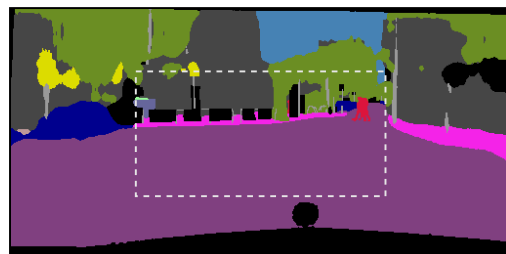

SPG-Net ++
